# Supplementary material for: Continual Learning with Extended Kronecker-factored Approximate Curvature
Source: arXiv:2004.07507 source file (2020-04-16)
Supplement: Supplementary file 1 [file supp.pdf]

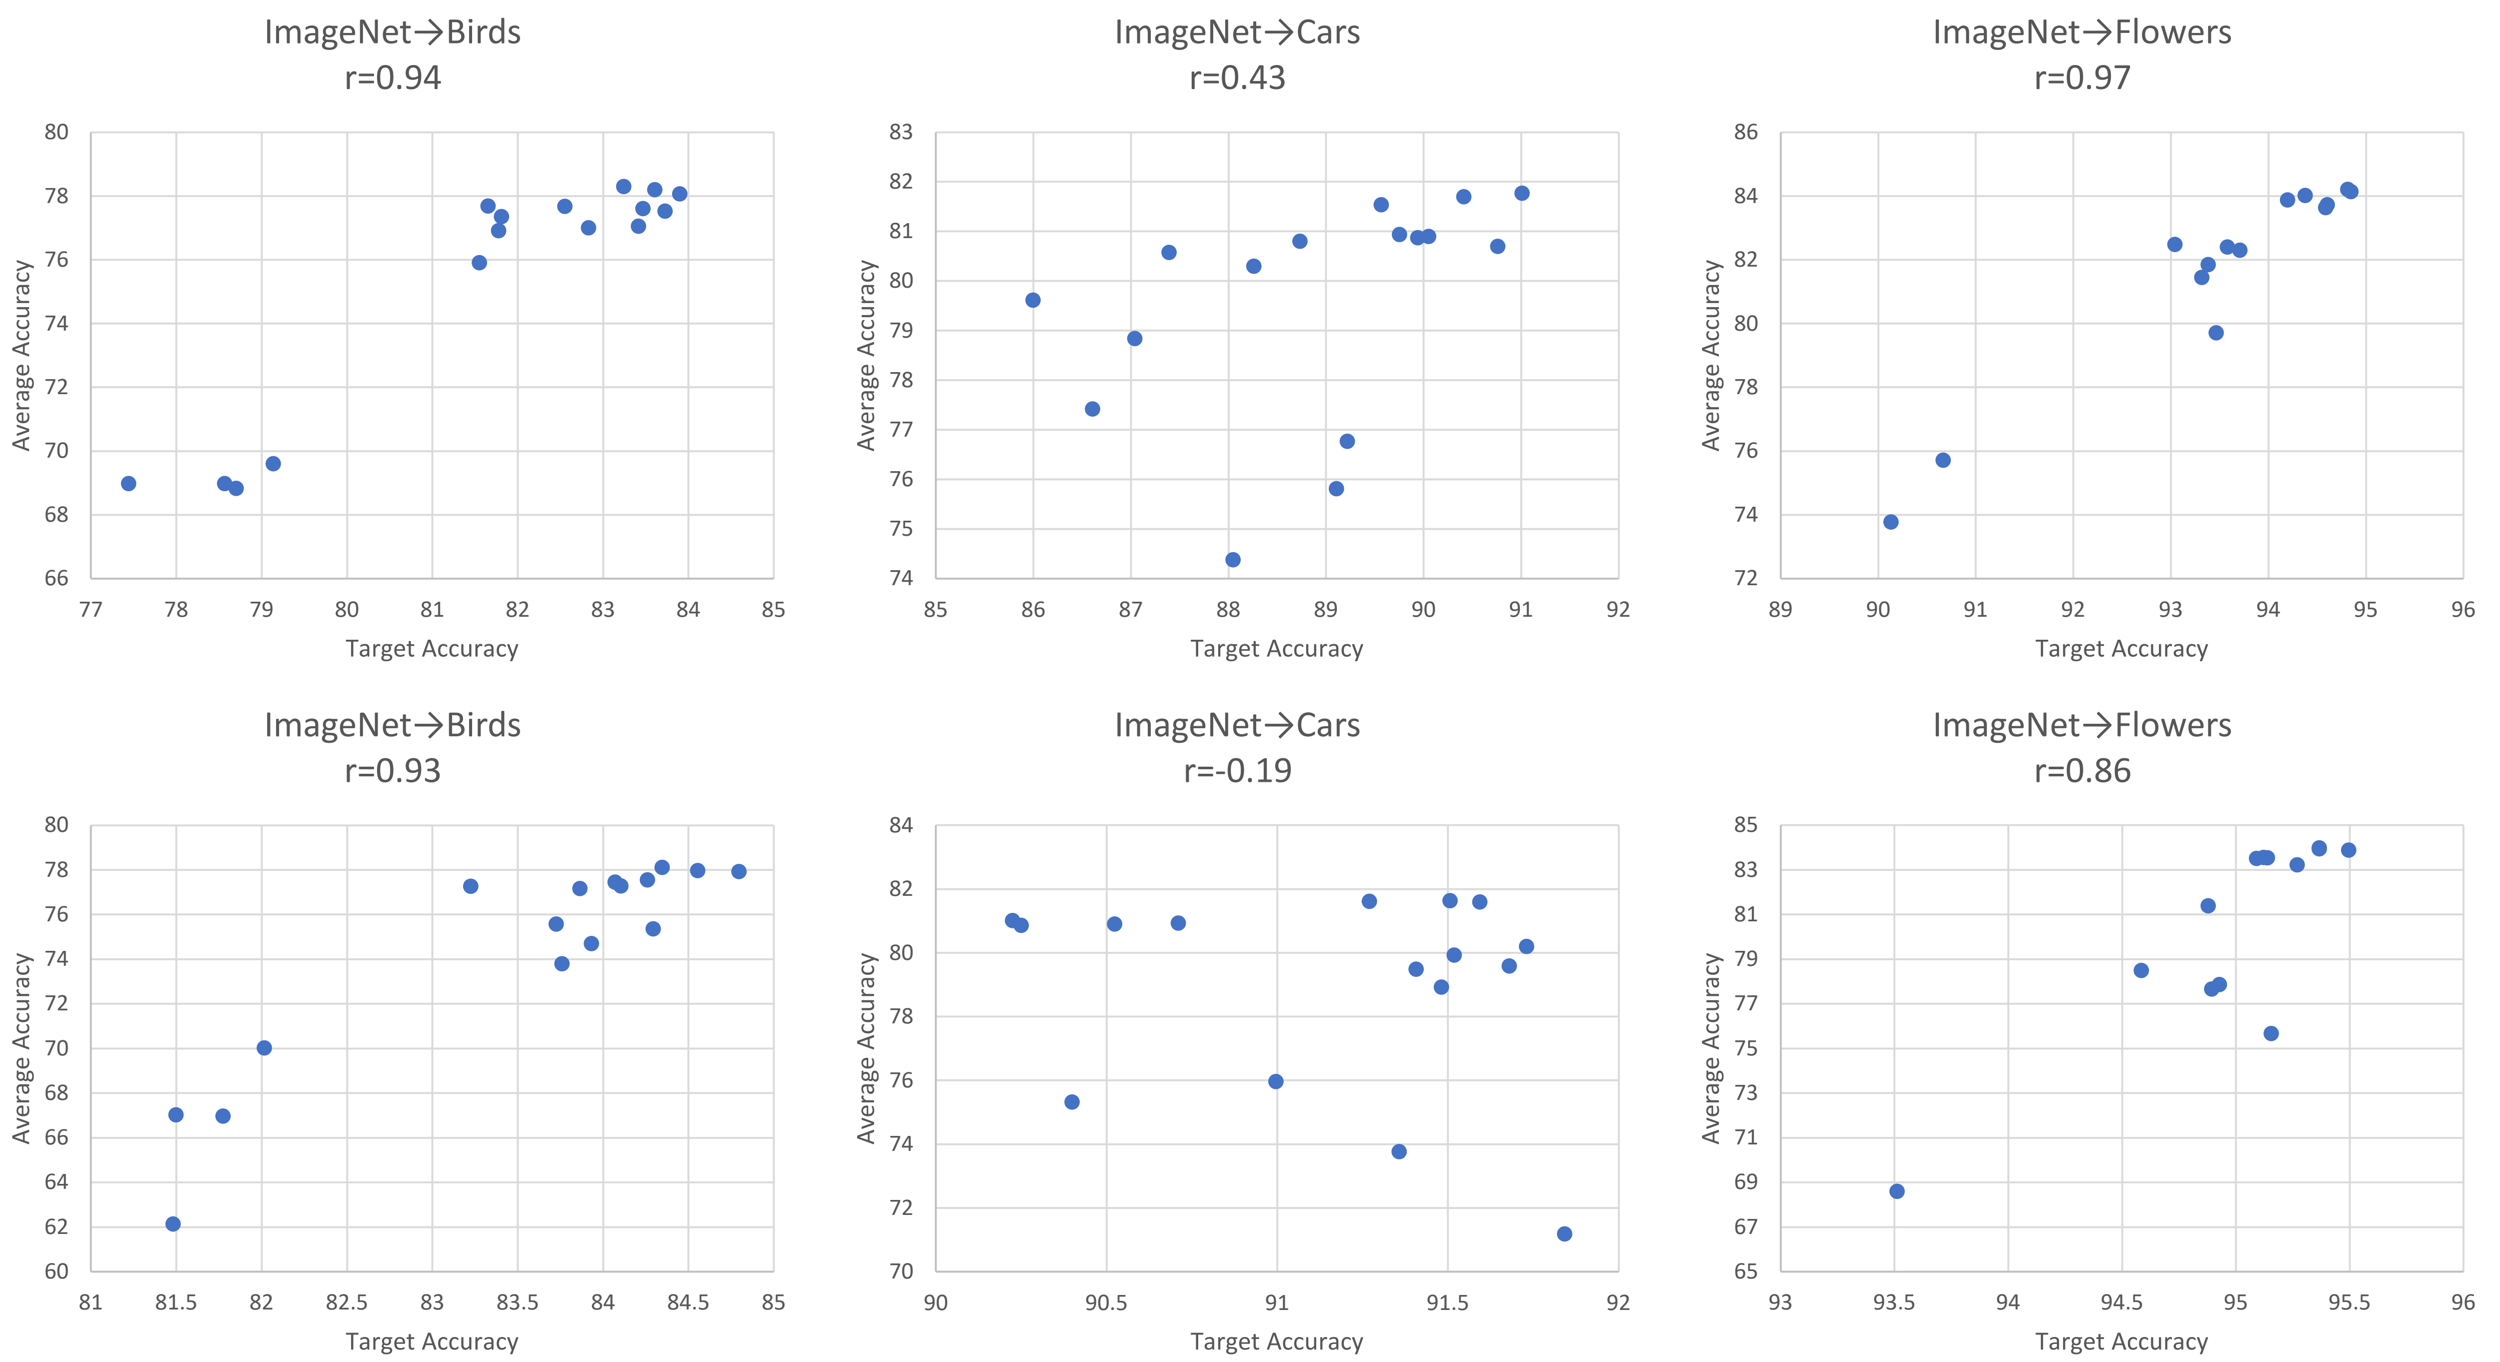

ImageNet→Birds
r=0.94
80
78
76
74
72
70
68
66
77
78
79
80
81
82
83
84
85
Average Accuracy
Target Accuracy
ImageNet→Cars
r=0.43
83
82
81
80
79
78
77
76
75
74
85
86
87
88
89
90
91
92
Average Accuracy
Target Accuracy
ImageNet→Flowers
r=0.97
86
84
82
80
78
76
74
72
89
90
91
92
93
94
95
96
Average Accuracy
Target Accuracy
ImageNet→Birds
r=0.93
80
78
76
74
72
70
68
66
64
62
60
81
81.5
82
82.5
83
83.5
84
84.5
85
Average Accuracy
Target Accuracy
ImageNet→Cars
r=-0.19
84
82
80
78
76
74
72
70
90
90.5
91
91.5
92
Average Accuracy
Target Accuracy
ImageNet→Flowers
r=0.86
85
83
81
79
77
75
73
71
69
67
65
93
93.5
94
94.5
95
95.5
96
Average Accuracy
Target Accuracy

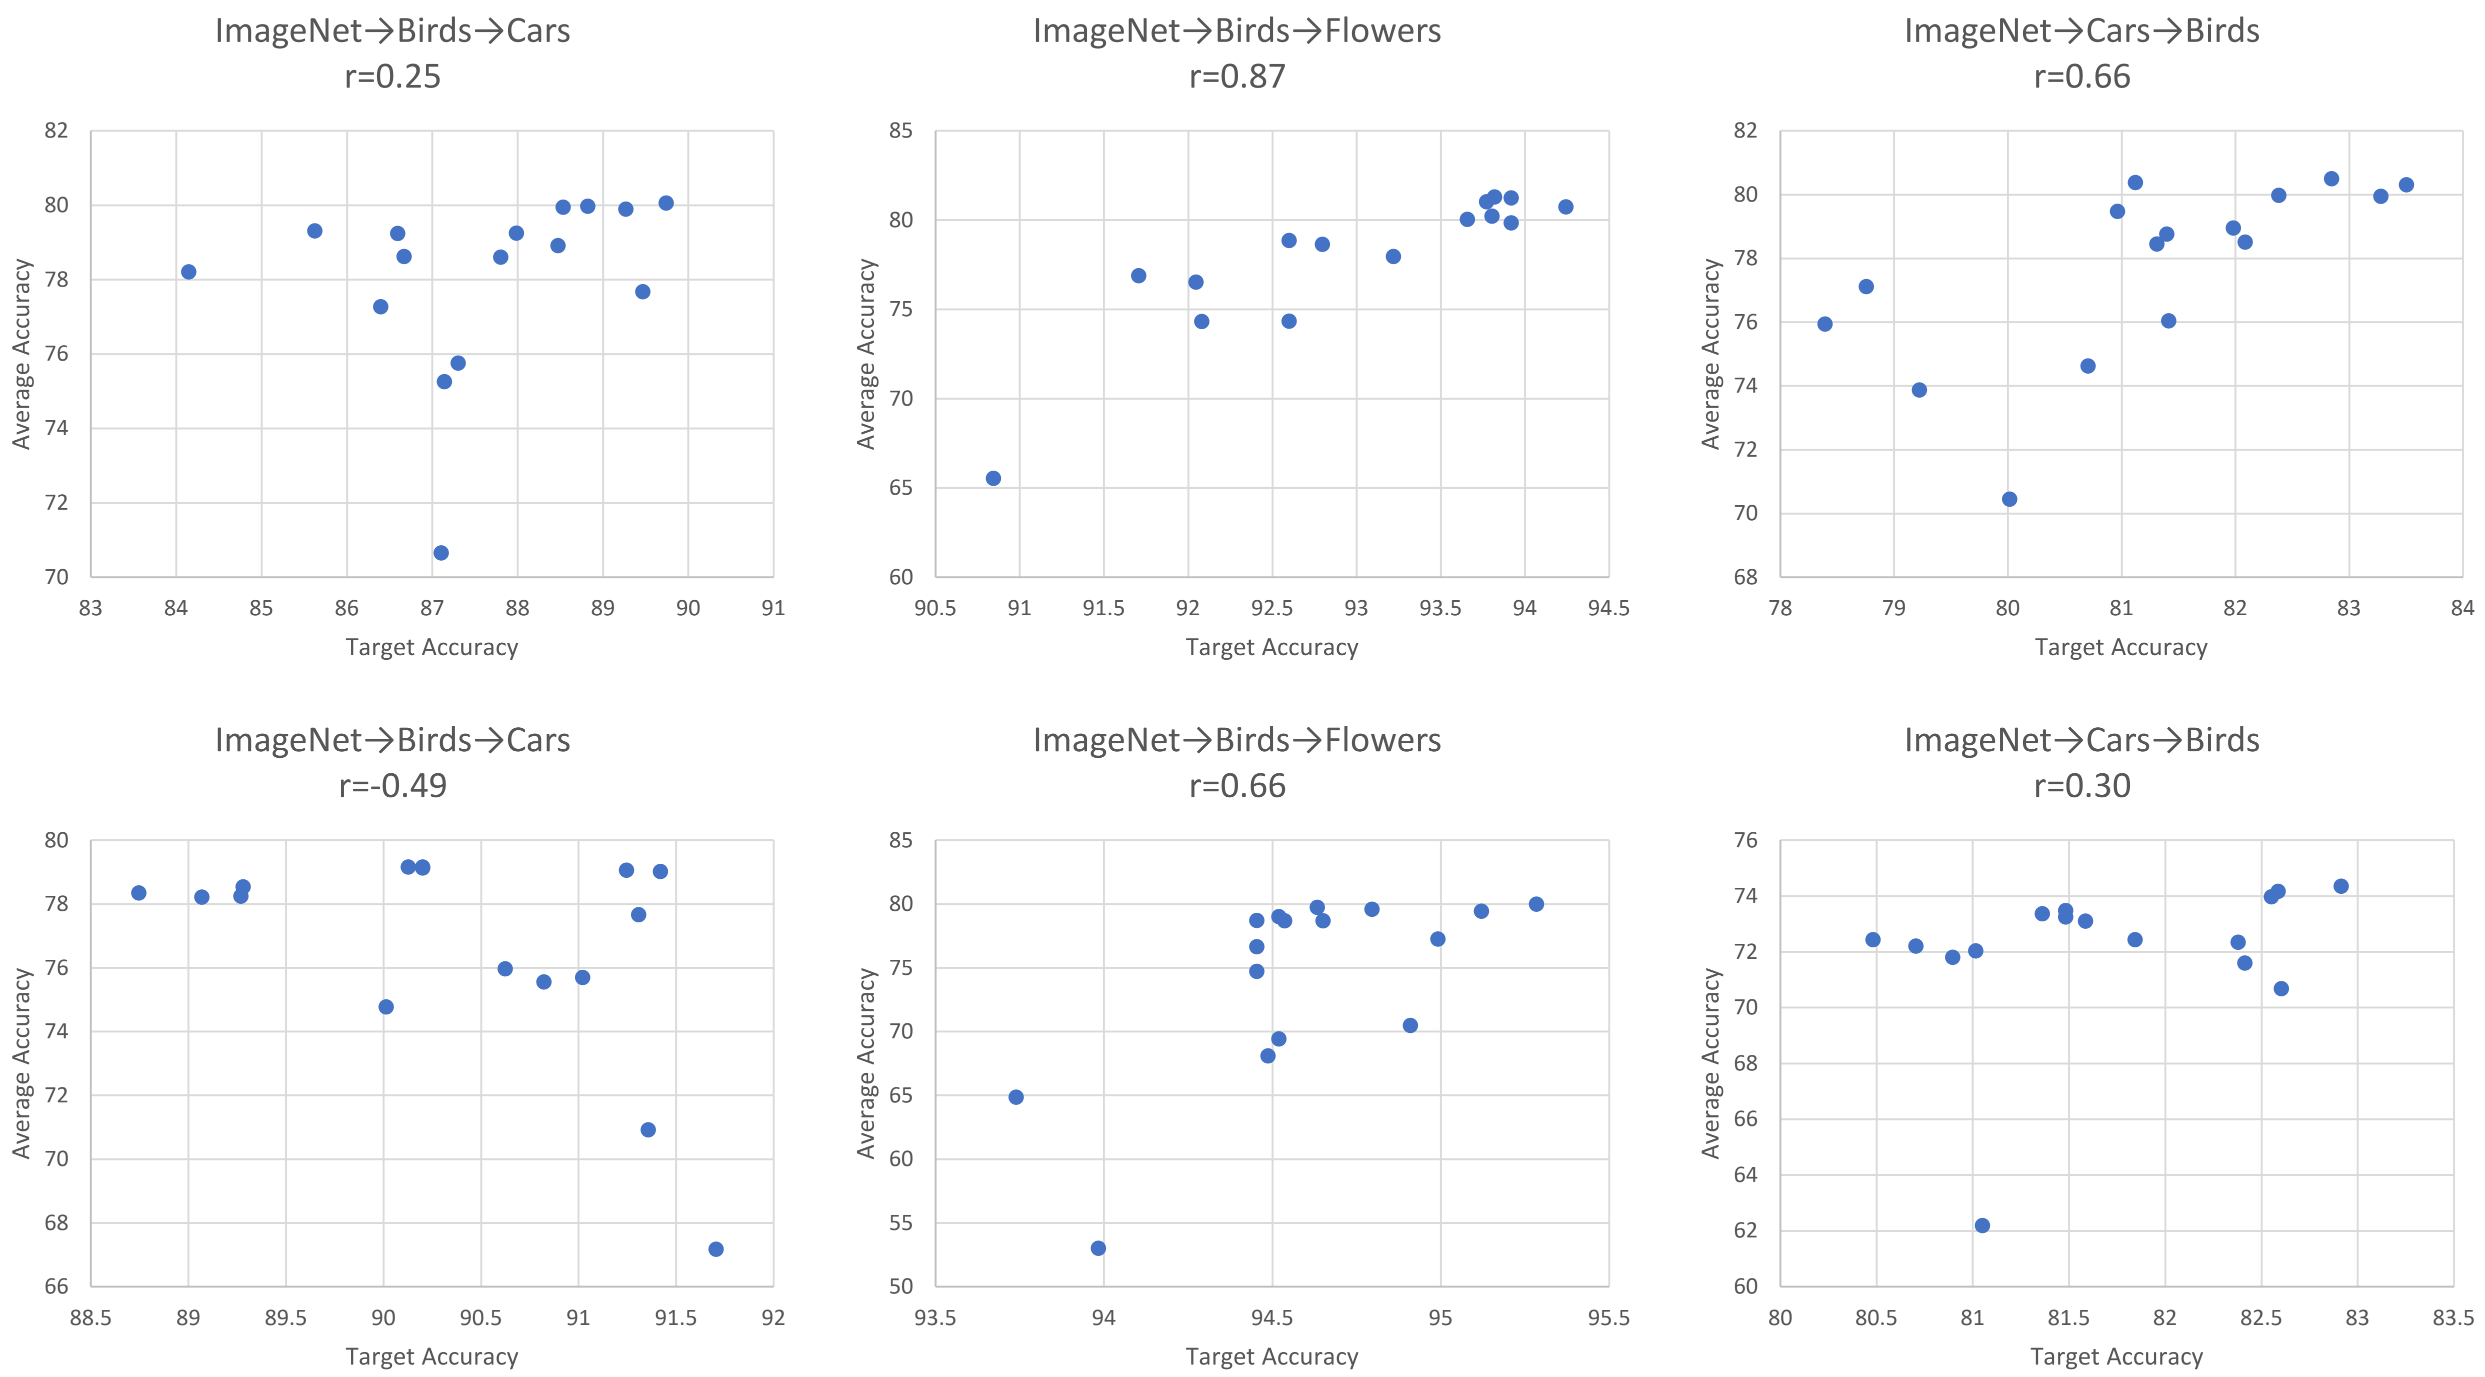
ImageNet→Birds→Cars
r=0.25
Average Accuracy
Target Accuracy
ImageNet→Birds→Flowers
r=0.87
Average Accuracy
Target Accuracy
ImageNet→Cars→Birds
r=0.66
Average Accuracy
Target Accuracy
ImageNet→Birds→Cars
r=-0.49
Average Accuracy
Target Accuracy
ImageNet→Birds→Flowers
r=0.66
Average Accuracy
Target Accuracy
ImageNet→Cars→Birds
r=0.30
Average Accuracy
Target Accuracy

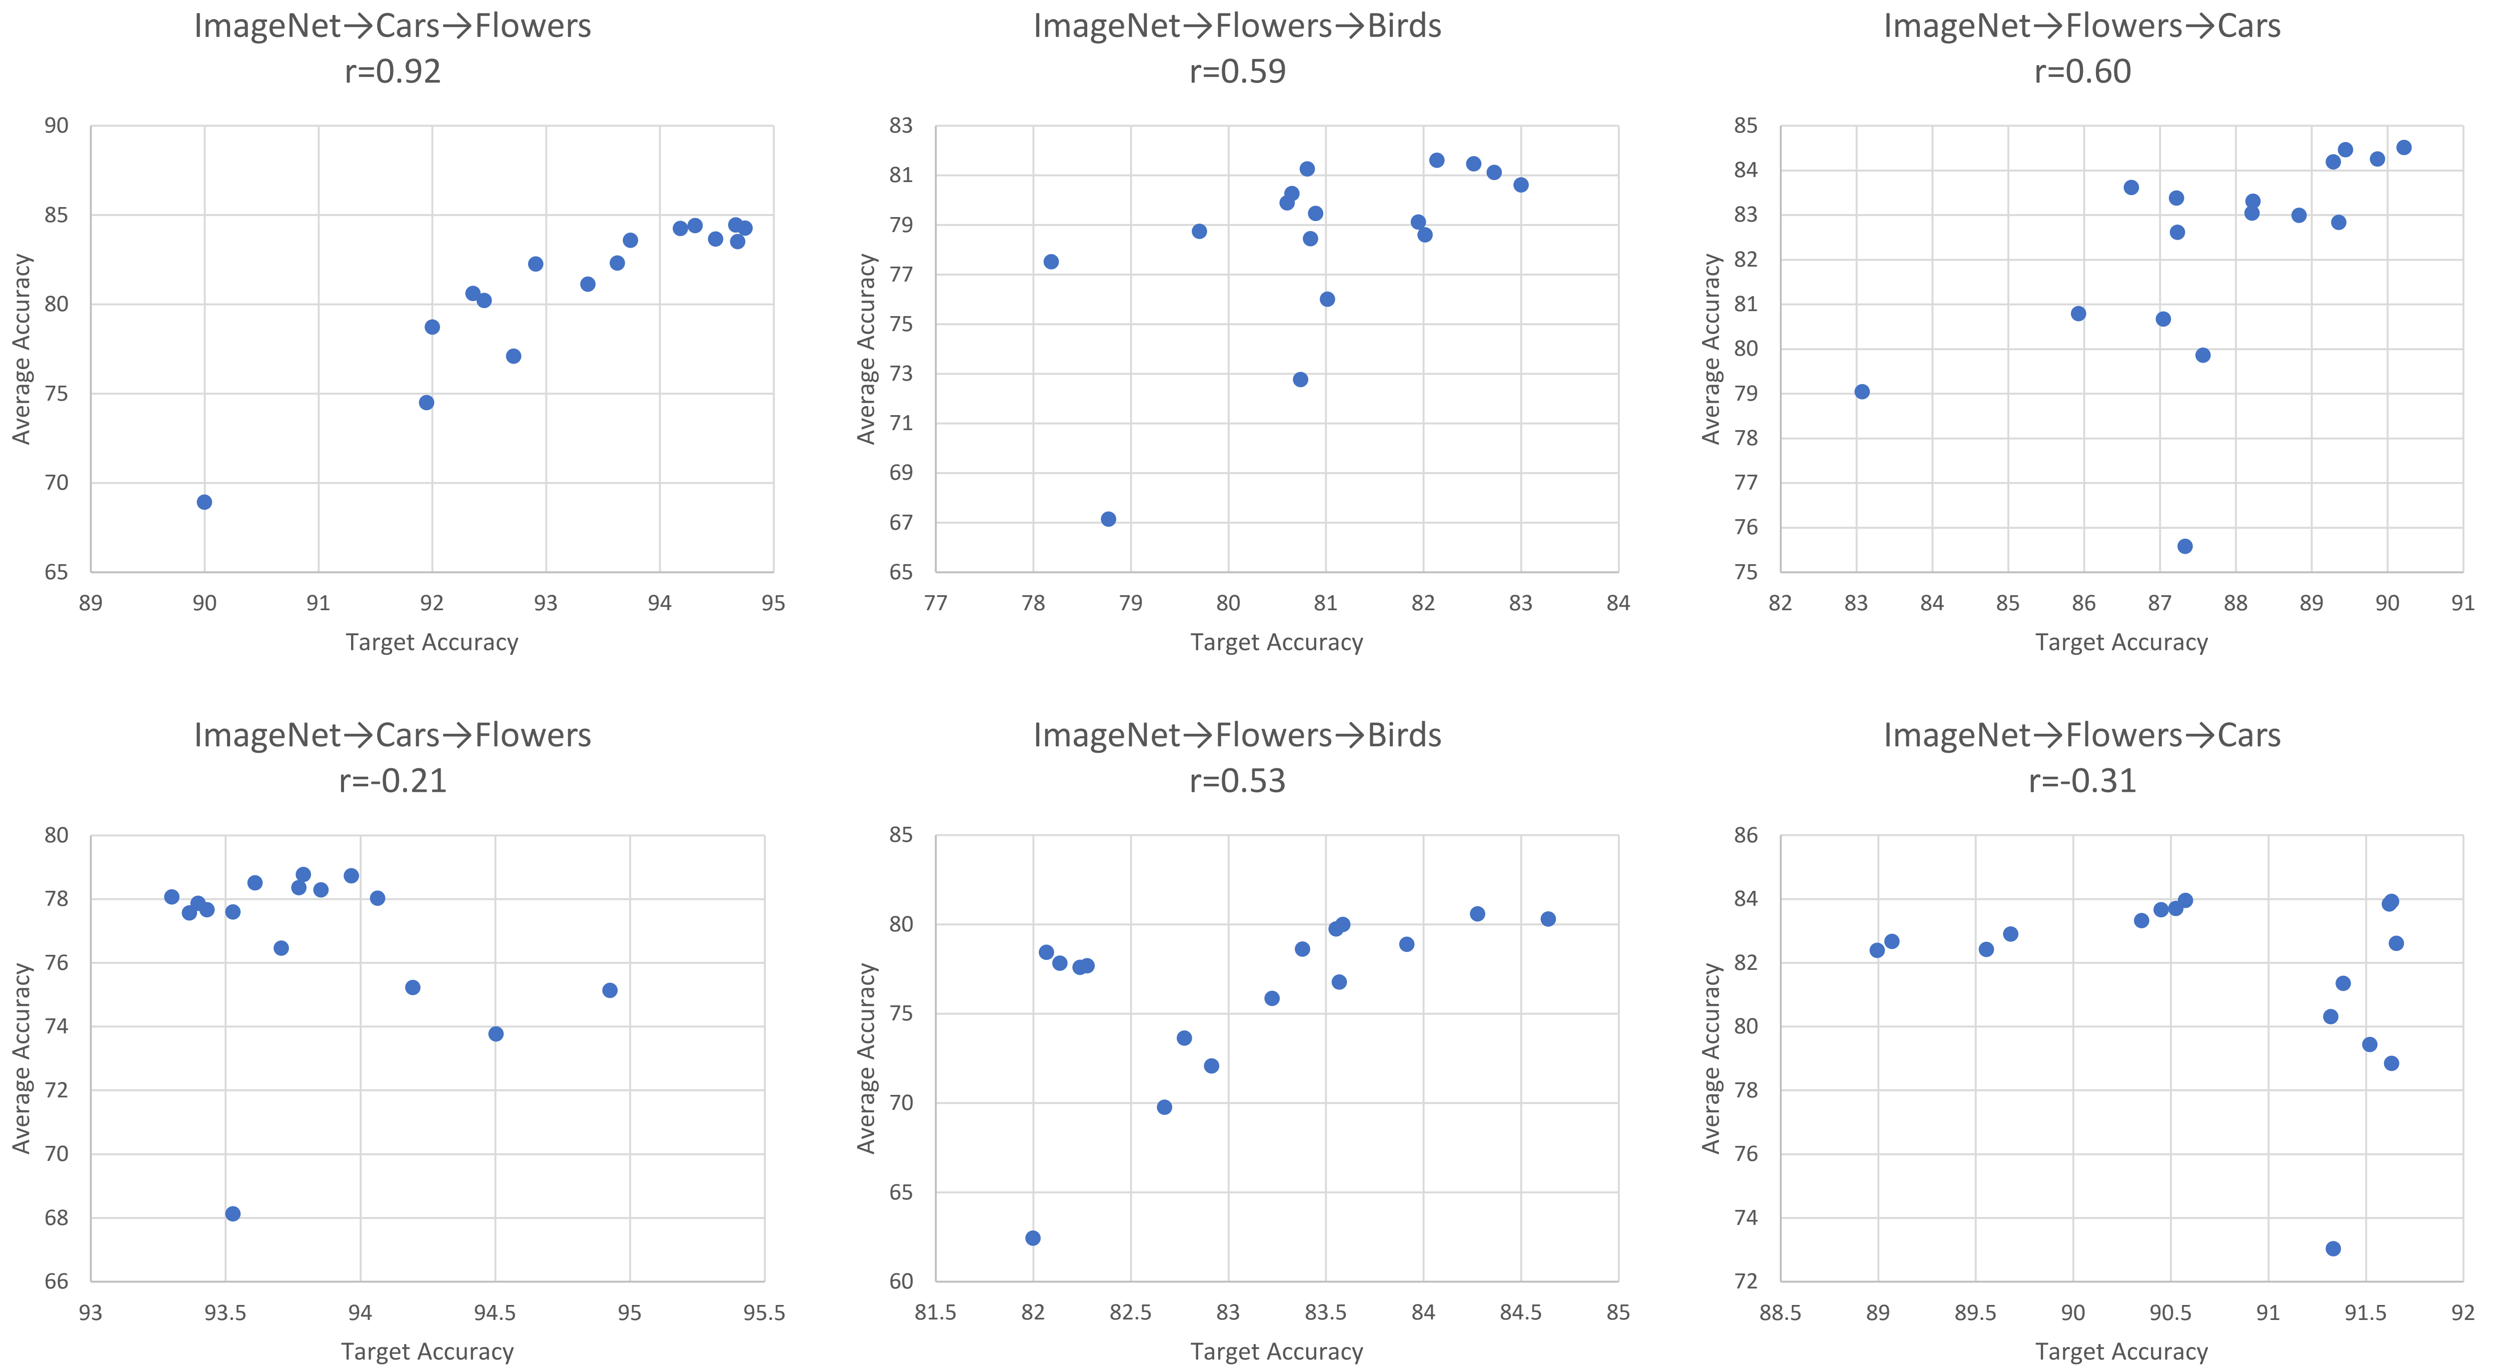
ImageNet→Cars→Flowers
r=0.92
Average Accuracy
Target Accuracy
65
70
75
80
85
90
89
90
91
92
93
94
95
ImageNet→Flowers→Birds
r=0.59
Average Accuracy
Target Accuracy
65
67
69
71
73
75
77
79
81
83
77
78
79
80
81
82
83
84
ImageNet→Flowers→Cars
r=0.60
Average Accuracy
Target Accuracy
75
76
77
78
79
80
81
82
83
84
85
82
83
84
85
86
87
88
89
90
91
ImageNet→Cars→Flowers
r=-0.21
Average Accuracy
Target Accuracy
66
68
70
72
74
76
78
80
93
93.5
94
94.5
95
95.5
ImageNet→Flowers→Birds
r=0.53
Average Accuracy
Target Accuracy
60
65
70
75
80
85
81.5
82
82.5
83
83.5
84
84.5
85
ImageNet→Flowers→Cars
r=-0.31
Average Accuracy
Target Accuracy
72
74
76
78
80
82
84
86
88.5
89
89.5
90
90.5
91
91.5
92

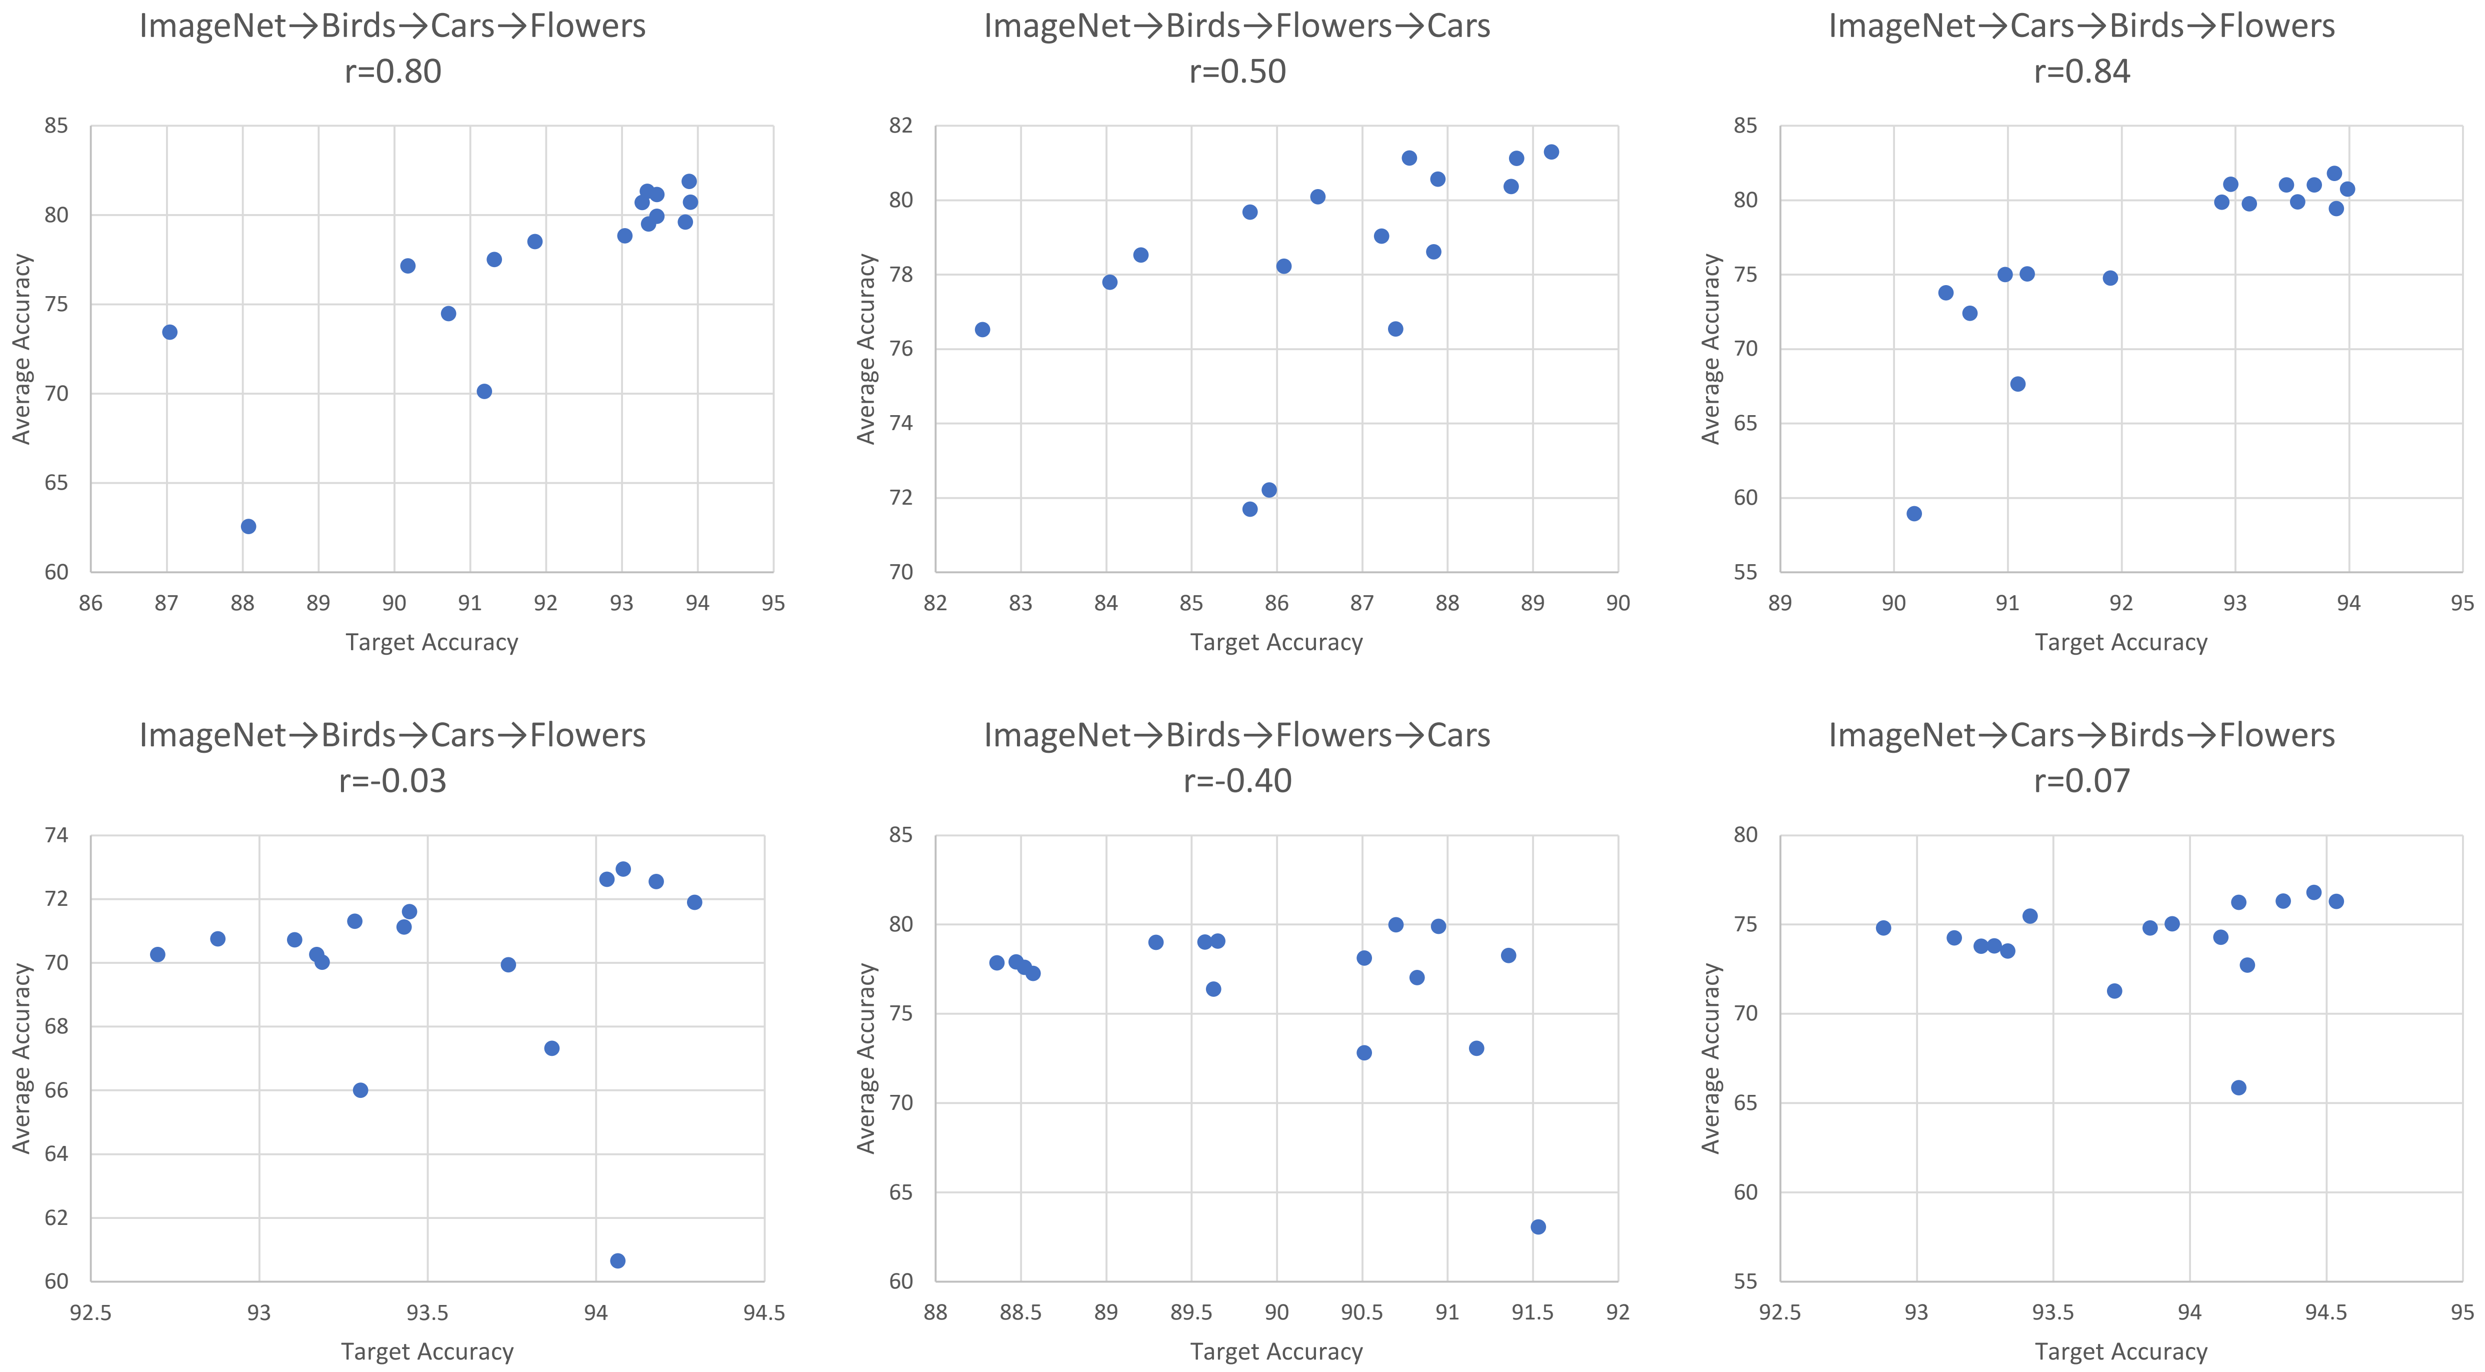
ImageNet→Birds→Cars→Flowers
r=0.80
Average Accuracy
Target Accuracy
ImageNet→Birds→Flowers→Cars
r=0.50
Average Accuracy
Target Accuracy
ImageNet→Cars→Birds→Flowers
r=0.84
Average Accuracy
Target Accuracy
ImageNet→Birds→Cars→Flowers
r=-0.03
Average Accuracy
Target Accuracy
ImageNet→Birds→Flowers→Cars
r=-0.40
Average Accuracy
Target Accuracy
ImageNet→Cars→Birds→Flowers
r=0.07
Average Accuracy
Target Accuracy

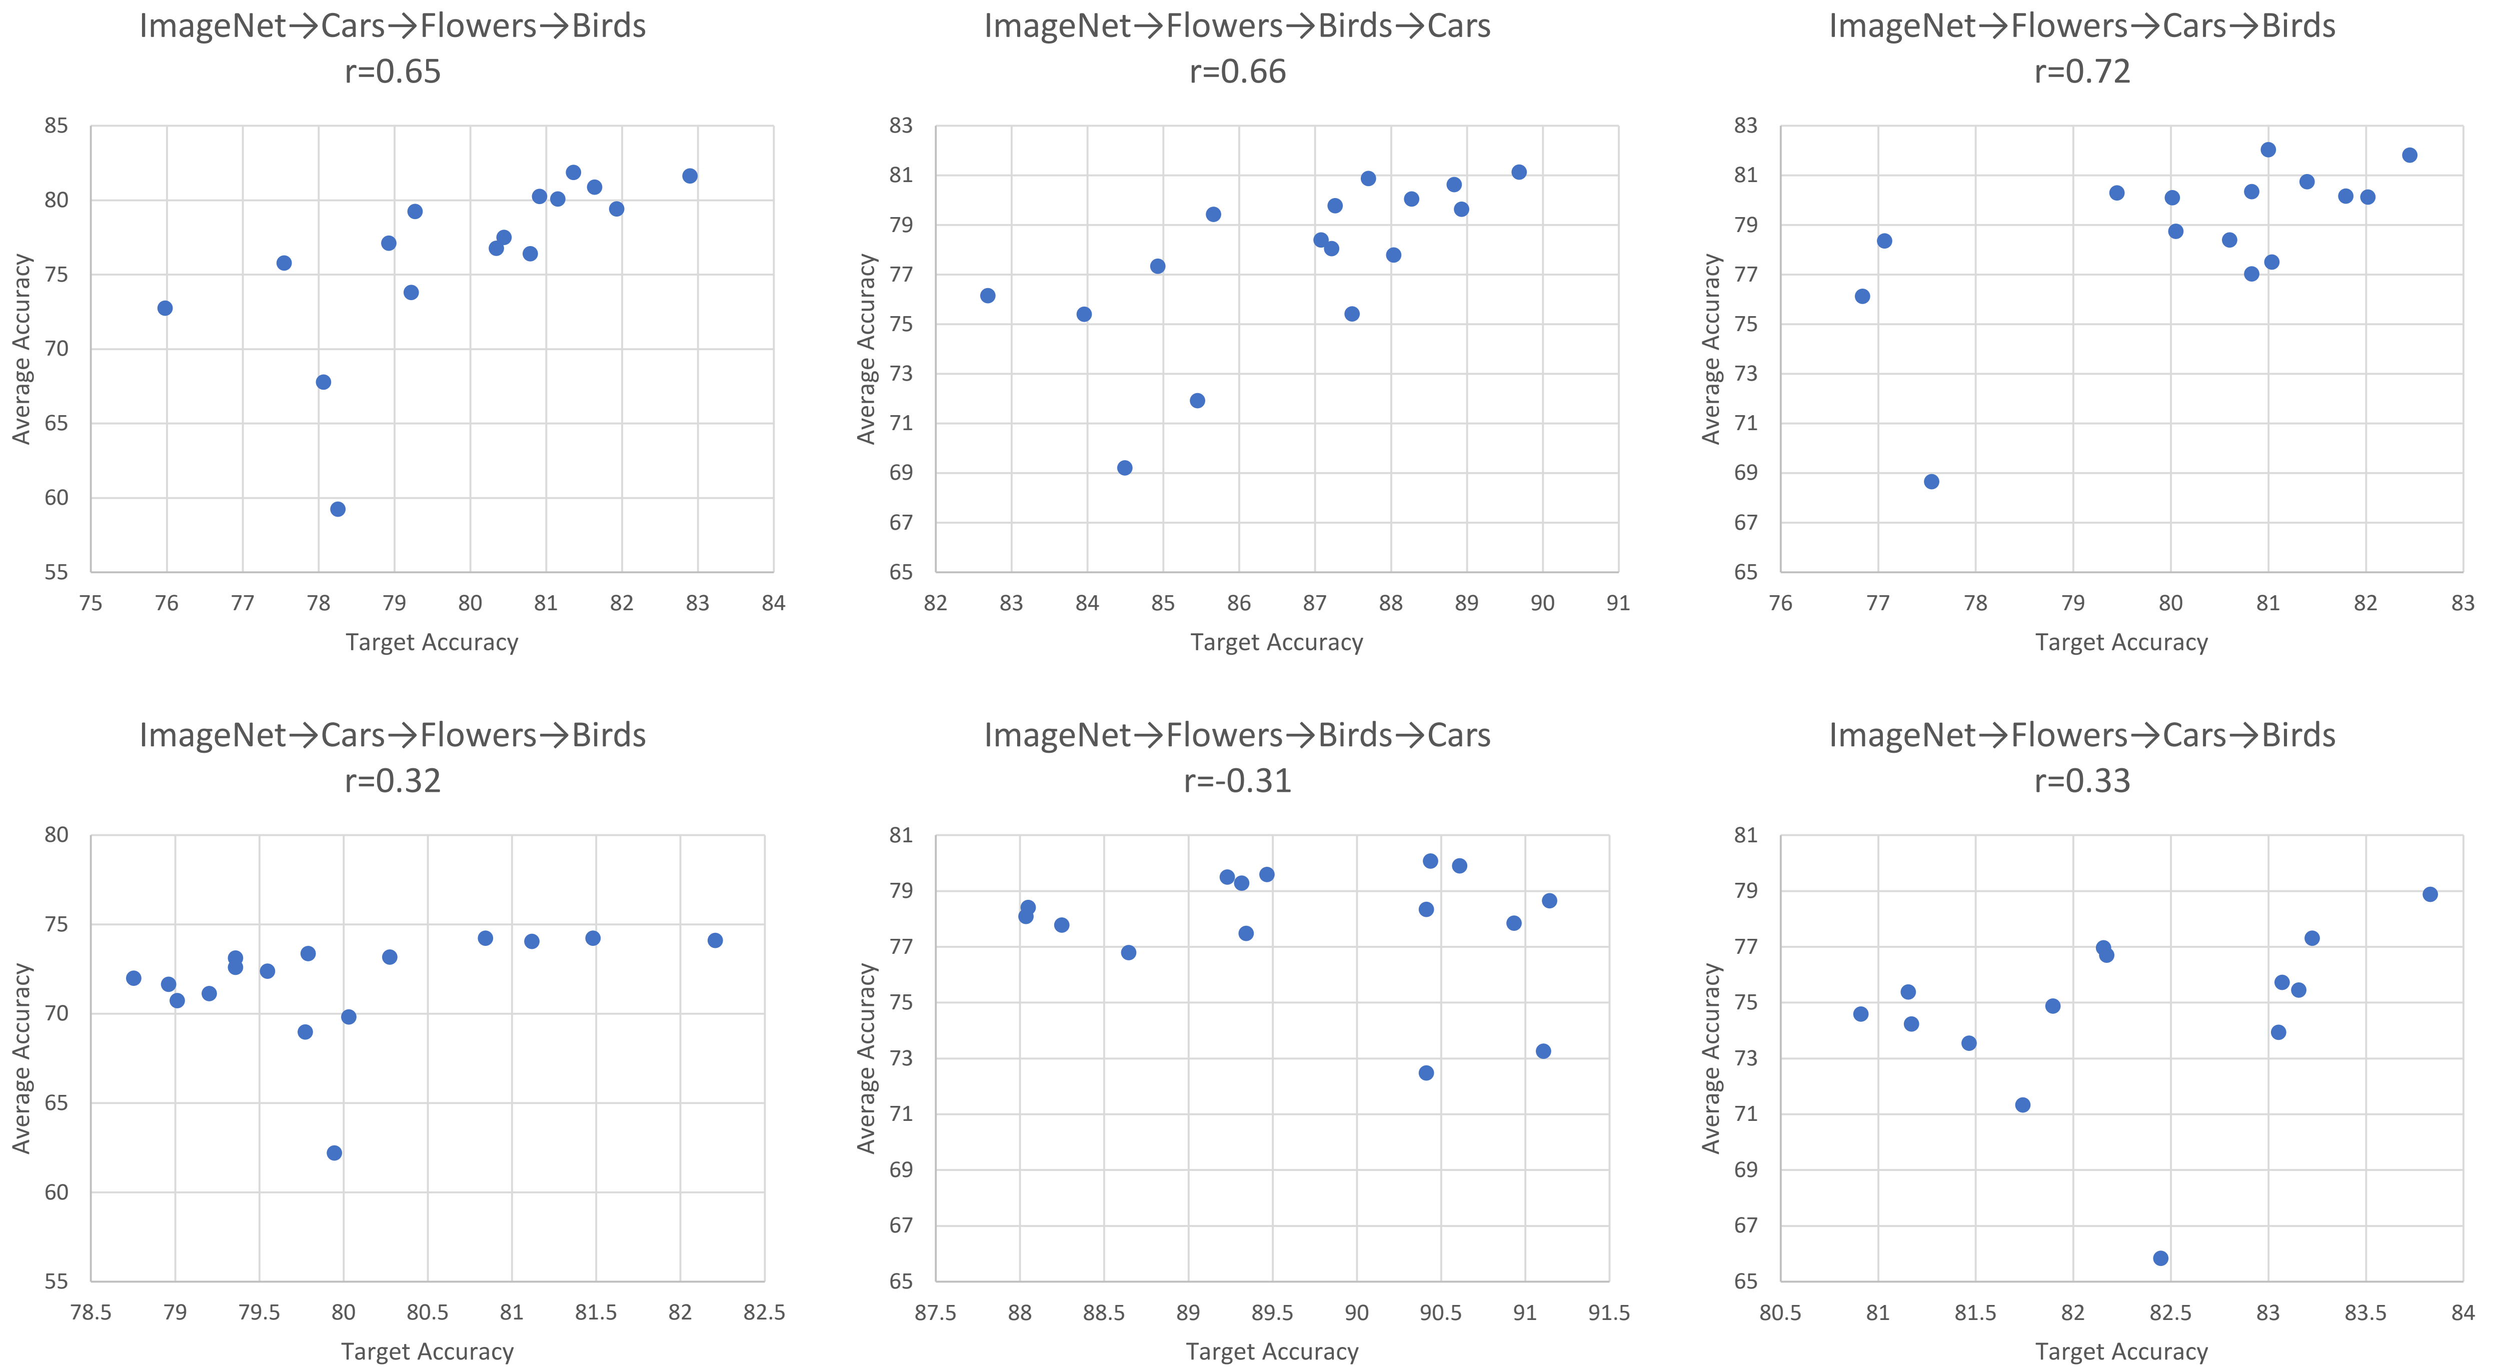
ImageNet→Cars→Flowers→Birds
r=0.65
Average Accuracy
85 80 75 70 65 60 55
75 76 77 78 79 80 81 82 83 84
Target Accuracy
ImageNet→Flowers→Birds→Cars
r=0.66
Average Accuracy
83 81 79 77 75 73 71 69 67 65
82 83 84 85 86 87 88 89 90 91
Target Accuracy
ImageNet→Flowers→Cars→Birds
r=0.72
Average Accuracy
83 81 79 77 75 73 71 69 67 65
76 77 78 79 80 81 82 83
Target Accuracy
ImageNet→Cars→Flowers→Birds
r=0.32
Average Accuracy
80 75 70 65 60 55
78.5 79 79.5 80 80.5 81 81.5 82 82.5
Target Accuracy
ImageNet→Flowers→Birds→Cars
r=-0.31
Average Accuracy
81 79 77 75 73 71 69 67 65
87.5 88 88.5 89 89.5 90 90.5 91 91.5
Target Accuracy
ImageNet→Flowers→Cars→Birds
r=0.33
Average Accuracy
81 79 77 75 73 71 69 67 65
80.5 81 81.5 82 82.5 83 83.5 84
Target Accuracy
